# Supplementary material for: Policy Choice in Time Series by Empirical Welfare Maximization
Source: arXiv:2205.03970 source file (2026-06-01)
Supplement: Supplementary file 2 [file Online_appendix.tex]

\documentclass[12pt,a4paper,english]{article}

\input{0_def}

%%%%%%%cross reference
\usepackage{xr}
\usepackage{hyperref}
\makeatletter
\newcommand*{\addFileDependency}[1]{% argument=file name and extension
	\typeout{(#1)}
	\@addtofilelist{#1}
	\IfFileExists{#1}{}{\typeout{No file #1.}}
}
\makeatother

\newcommand*{\myexternaldocument}[1]{%
	\externaldocument{#1}%
	\addFileDependency{#1.tex}%
	\addFileDependency{#1.aux}%
}
\myexternaldocument{main_4.0}
\myexternaldocument{Online_appendix_B}
\hypersetup{linkcolor={blue}}

%\newcommand{\hint}[1]{\textcolor{hint}{\texttt{#1}}}
%%%%%%%%%

%\title{\Large{\textbf{Appendix A of \textquotedblleft Policy Choice in Time Series by Empirical Welfare Maximization\textquotedblright}\Large 
		%\thanks{We are grateful to Karun Adusumilli, Isaiah Andrews, Giuseppe Cavaliere, Yoosoon Chang, Wei Cui, Whitney Newey, Joon Park, Barbara Rossi, Frank Schorfheide, and  the participants at the EEA-ESEM 2021, IAAE Annual Meeting 2022, and seminars at CeMMAP, Indiana University, Philadelphia Fed, TEDS, University of Carlos III Madrid, University of Glasgow, University of Notre Dame, and University of Oxford for beneficial comments. We are grateful to Thomas Carr for his excellent research assistance.  Financial support fromthe ESRC through the ESRC CeMMAP (grant number RES-589-28-0001) and the ERC (grant number 715940) is gratefully acknowledged. Weining Wang's research is partially supported by the ESRC (Grant Reference: ES/T01573X/1).}
%	}}
%\author{Toru Kitagawa\thanks{Department of Economics, Brown University and Department of Economics, University College London. Email: toru\_kitagawa@brown.edu} \hspace{0.5cm} Weining Wang\thanks{Department of Economics and Related Studies, University of York. Email: weining.wang@york.ac.uk} \hspace{0.5cm} Mengshan Xu\thanks{Department of Economics, University of Mannheim. Email: mengshan.xu@uni-mannheim.de}}
\begin{document}
	\onehalfspacing
	\date{}
	%\maketitle
\appendix
\numberwithin{equation}{section}
\input{9_appendix_1}
\bibliographystyle{abbrvnat}
\bibliography{biball}
\end{document}
